# Supplementary material for: Adaptive Compliance Policy: Learning Approximate Compliance for Diffusion Guided Control
Source: arXiv:2410.09309 source file (2025-03-07)
Supplement: Supplementary file 1 [file appendix.tex]

\newpage
\section*{APPENDIX}

\begin{figure*}
    \centering
    \includegraphics[width=0.9\linewidth]{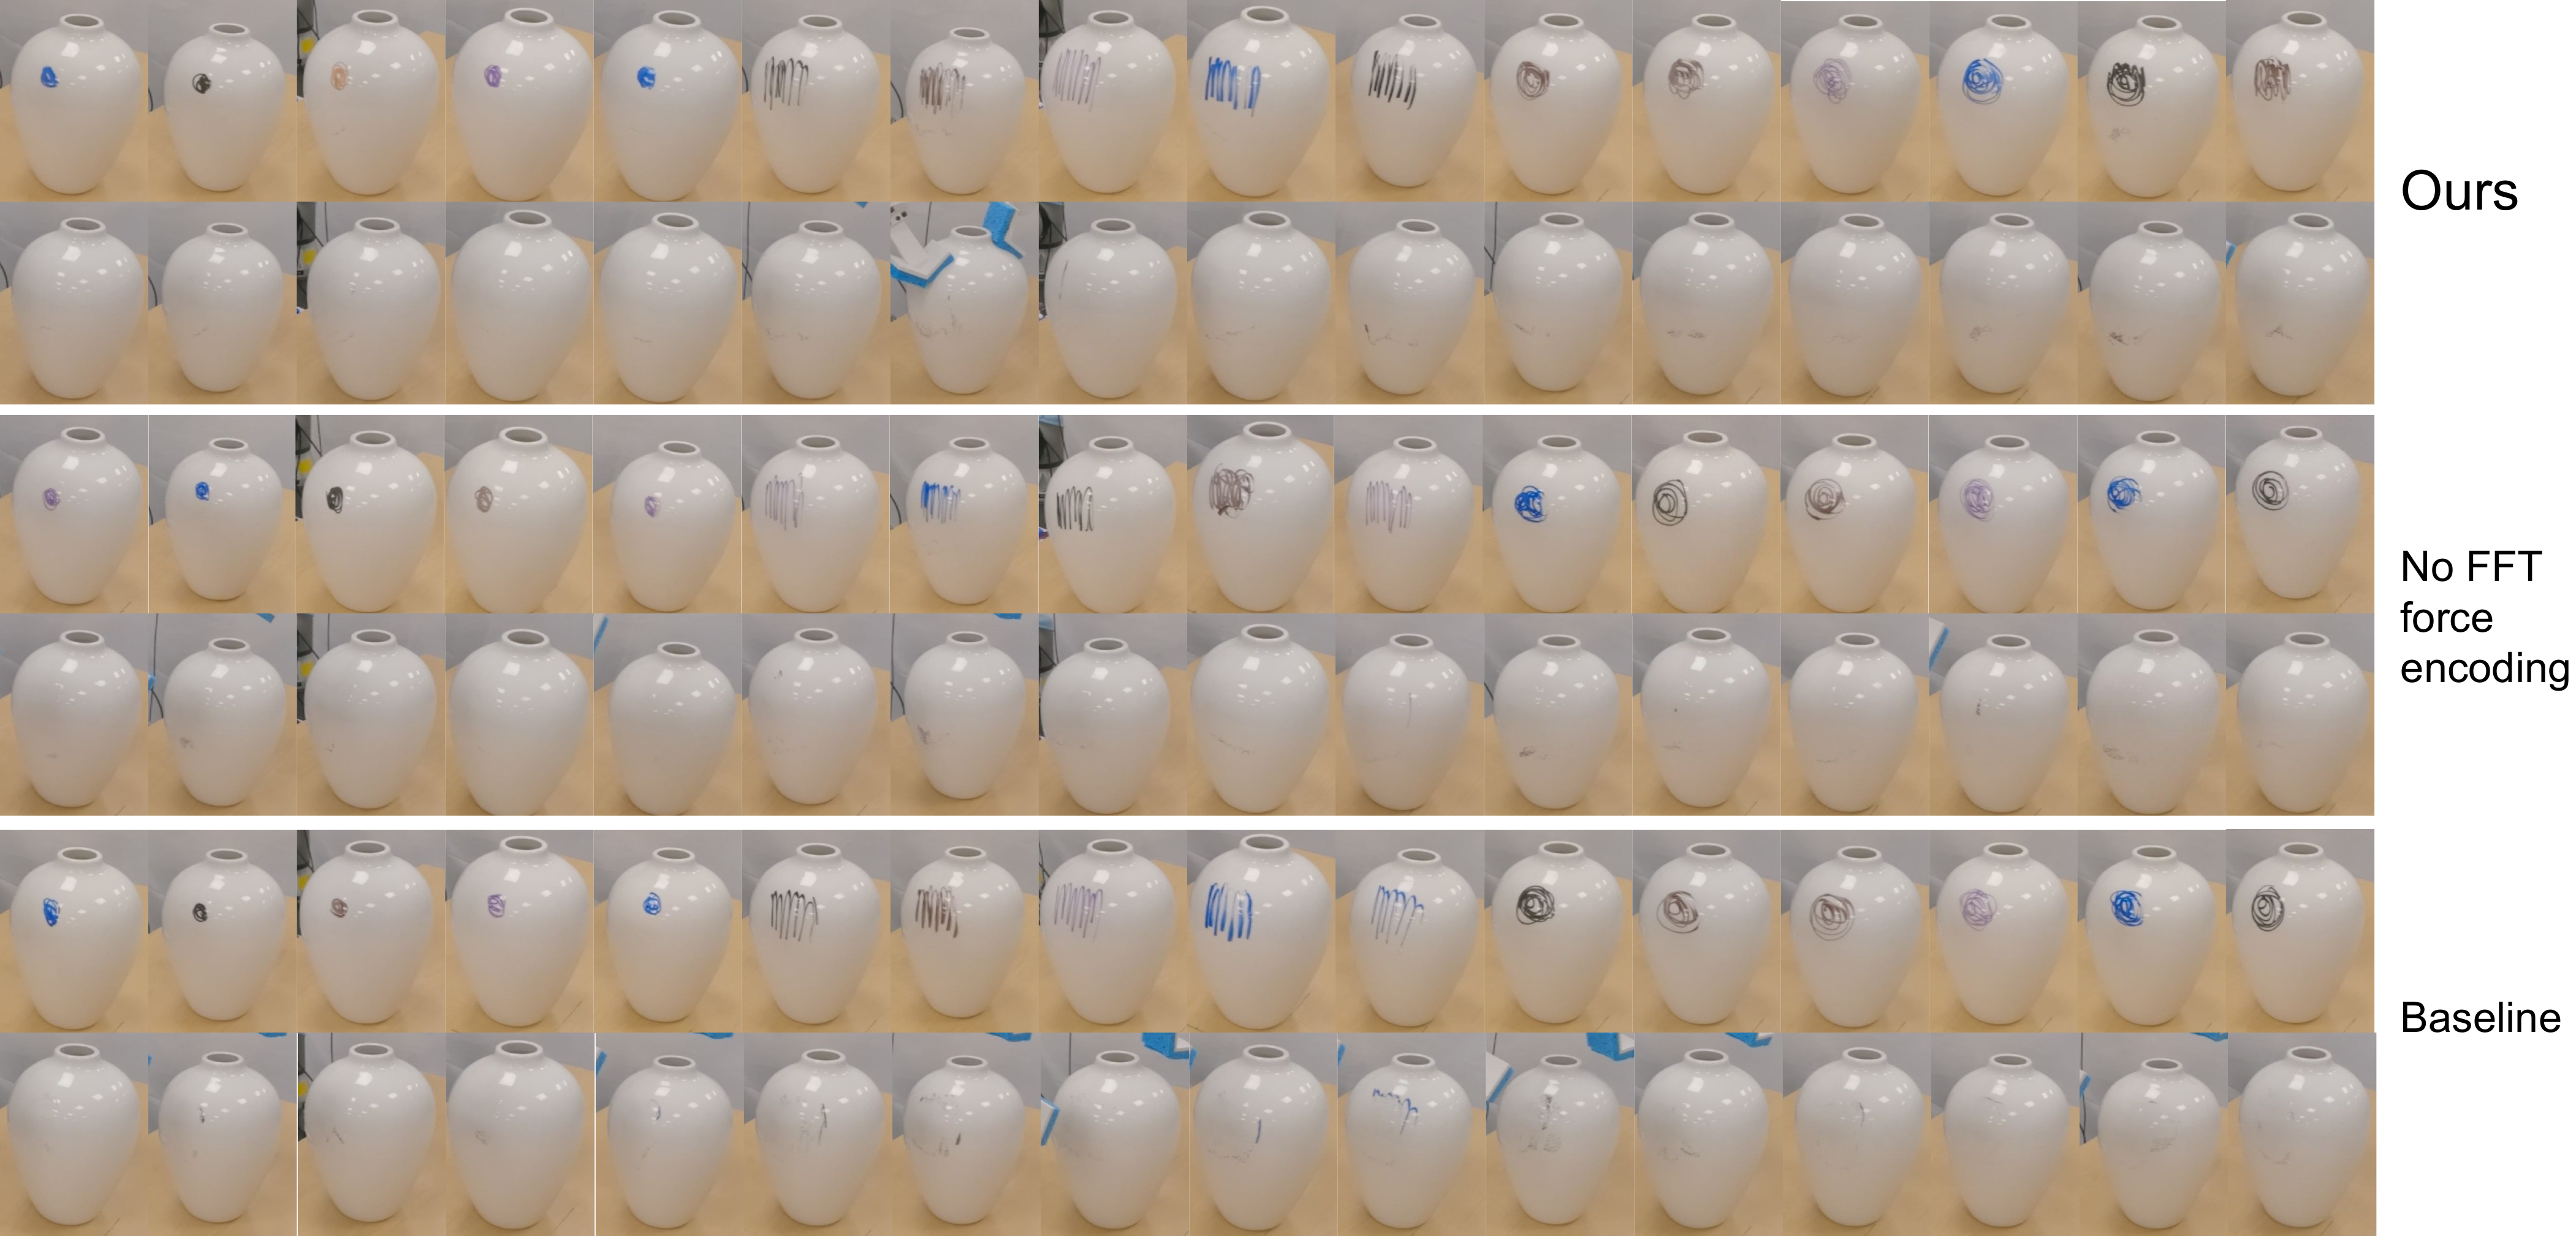}
    \caption{\textbf{Wiping Result.} In each group, the top row shows the initial state of the vase, the bottom row shows the result after up to three wipes. Top group: our method wiped every vase clean except for the eighth one. Middle group: result of the ablation study where force encoding is replaced with a temporal convolution network. Bottom group: result of the uniform compliance baseline.}
    \label{fig:wiping_result_detailed}
    % https://docs.google.com/drawings/d/1UhRB5DqcENhL5lYb-EWVp5vyQLQOQV6wfIHd3bbaTGs/edit?usp=sharing
\end{figure*}

For consistency between evaluations, we always orient the marking to the right of the robot and initialize the robot to the same pose. The vase position of each test is shown in Fig. \ref{fig:wiping_test_layout}.

\begin{figure}[h]
    \centering
    \includegraphics[width=0.8\linewidth]{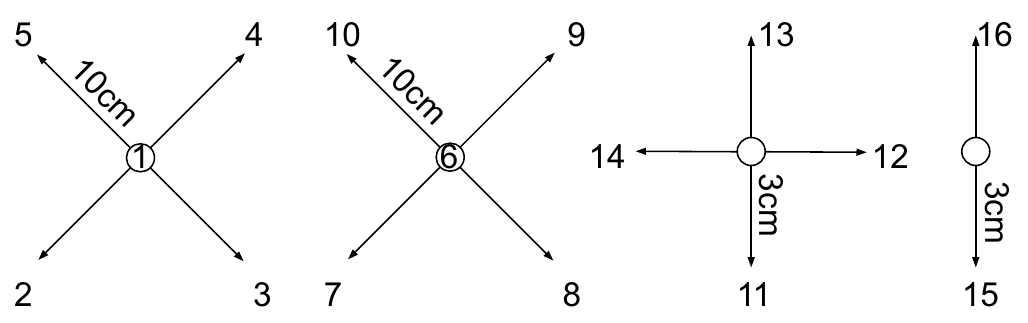}
    \caption{Vase locations for each of the test scenario. In each scenario, the center circle represents the nominal vase location that the demonstrations were collected around. \vspace{-3mm}}
    \label{fig:wiping_test_layout}
    % https://docs.google.com/drawings/d/1QGgFGaG8zgrbwUPVart8gL3gvQTxZL-ceMKvuMXIncA/edit
\end{figure}

\begin{table}[ht]
\centering
\caption{Vase wiping test success rates with respect to number of wipes}
\label{tb:wiping_result}
\begin{tabular}{l|l|l|l}
\toprule 
Success rate after: & One wipe & Two wipes & Three wipes \\  
ACP                 & 12.5\%   & 56.25\%   & 93.75\%     \\  
ACP w.o. FFT        & 6.25\%   & 43.75\%   & 81.25\%     \\  
Compliant Policy    & 6.25\%   & 31.25\%   & 50\%        \\  
Stiff Policy        & N/A      & N/A       & N/A         \\  
\bottomrule  
\end{tabular}
\end{table}
